# Supplementary material for: Conditional Neural Architecture Search
Source: arXiv:2006.03969 source file (2020-06-06)
Supplement: Supplementary file 1 [file 09-Appendix.tex]

\section{Appendix}

%\section{Discussion and Future work}

\subsection{Discussion and Future work}

\textbf{More descriptive representations of the network.}
We use the network descriptor with nodes per layer and bits per layer. However, more descriptions can be Incorporated to genereate richer representations of the network. For example, we could enable pruning by adding pruning percentage per layer. We could also tune more model hyper-parameter such as types of activation function, dropout rate, number of epochs and learning rate. While these provides a more complete representation of the network, they increase the search space and the complexity that the GAN would have to encounter. There may be new considerations that have to be incorporated into the training of the generator to capture the increase in complexity.

\textbf{Pruning and quantization from pre-trained model.}
We expect the developed framework can be applied to optimize the pre-trained model by learning the pruning and quantization strategy. The presented generative method could be an alternative to the reinforcement learning-based methods \cite{he2018amc, wang2019haq} to compress DNN model.

\textbf{Electronics Design Autonomy.}
We expect the full automation of hardware deployment, which minimizes the effort required from a EDA engineer completely automating the hardware deployment process. We expect the device-aware neural network description generated from INAG to be an input of ML high level synthesis EDA tools \cite{duarte2018fast}, in our future work. Finally, after the generative model is tuned and trained by ML experts, the hardware-optimized neural network could be automatically deployed. 

We leave these three directions as our future work.
